# Supplementary material for: Valley-Polarized Exciton-Polaritons in a Monolayer Semiconductor
Source: arXiv:1701.05579 ancillary file (2017-01-19)
Supplement: Supplementary file 1 [file Chen_2017_SupplementaryInformation.pdf]

# Supplementary Material for Valley-Polarized Exciton-Polaritons in a Monolayer Semiconductor

Yen-Jung Chen,[1] Jeffrey D. Cain,[2,3] Teodor K. Stanev,[1] Vinayak P. Dravid,[2,3] and Nathaniel P. Stern[1]

[1] *Department of Physics and Astronomy, Northwestern University, Evanston, Illinois 60208 USA*

[2] *Department of Materials Science and Engineering, Northwestern University, Evanston, Illinois 60208, USA*

[3] *International Institute for Nanotechnology, Northwestern University, Evanston, Illinois 60208, USA*

## I. SAMPLE FABRICATION

Monolayers of $MoS_2$ were synthesized using atmospheric pressure chemical vapor deposition (CVD). The growth scheme proceeds as follows [1]. Powdered transition metal oxides, $MoO_3$, served as the transition metal source. 10 mg of the oxide precursor was placed in an alumina boat at the center of a 12 in. tube furnace with a 1 in. diameter quartz tube, while a clean Si wafer with a 300 nm $SiO_2$ capping layer was suspended, face down, above the boat (∼1 cm). 135 mg of sulfur powder was placed upstream in a lower temperature zone of the furnace and then heated to evaporation. The furnace temperature was raised, at a rate of 20 °C/min, to 700 °C and held there for 3 minutes. The furnace was switched off and allowed to cool to room temperature naturally before removing the substrate. During this entire process ultra-high purity Ar gas was flowed at a rate of 15 sccm regulated using a mass flow controller to act as a carrier gas for sulfur vapor.

The CVD-synthesized monolayer $MoS_2$ on Si/$SiO_2$ has flake size around 10 $\mu$m as measured under an optical microscope (Fig. S1a). The flakes have the expected triangular shape with a thickness of 0.8 nm measured by atomic force microscopy (AFM) (Fig. S1b). Raman spectroscopy shows characteristic splitting of a monolayer $MoS_2$ between the $E^1_{2g}$ and $A_{1g}$ peaks at about 20 cm$^{-1}$ (Fig. S1c).

For the microcavity (MC) fabrication (Fig. S1d), a bottom DBR was deposited on a silicon chip using plasma-enhanced chemical vapor deposition (PECVD). Alternating layers of $SiO_2$ and $Si_3N_4$ with thickness of $\lambda/4n$ were deposited to constitute a distributed Bragg reflector (DBR). Monolayer $MoS_2$ was transferred from a Si/$SiO_2$ chip onto the bottom DBR. The top DBR was then deposited using the same method as the bottom. The inner layer of each DBR surrounding the monolayer $MoS_2$ is $SiO_2$.

The CVD-grown monolayer $MoS_2$ was transferred into the DBR MC using a polycarbonate (PC) transfer technique [2–4]. The original chip with the CVD-grown monolayers was lightly coated with 5% PC in chloroform (by mass) and spun at 1600 RPM to create a thin layer over the entire surface. The sample was heated briefly for one minute at 120°C to promote

good adhesion between the film and the monolayer. The film was then carefully peeled off and positioned over the bottom DBR. The film was melted gradually onto the bottom DBR through a series of heating processes (50°C for 1 minute, 100°C for 2 minutes, and 150°C for 10-15 minutes) and then submerged into chloroform to wash away the PC residue. The DBR was rinsed with acetone and isopropyl alcohol before being annealed for three hours at 350°C in an argon environment at atmospheric pressure to burn away any organic residue.

## II. OPTICAL CHARACTERIZATION

Angle-resolved reflectivity was performed using a vertically-oriented goniometer with resolution of 1° (Fig. S1e). White light from a fiber-coupled stabilized tungsten-halogen source (Thorlabs) was collimated and focused onto the sample using a lens with 12 cm focal length. The beam divergence from the lens to the sample was 2° and the final spot size was measured as $\sim$200 $\mu$m. Reflected light was collimated and collected into a fiber-coupled grating spectrometer (Andor Shamrock 303i) with a CCD yielding 0.5 nm spectral resolution.

Standard photoluminescence (PL) characterization on bare monolayer $MoS_2$ was done with a 532 nm CW diode laser (SpectraPhysics Millennia). The pump laser was focused onto the monolayer sample with both an objective (spot size of $\sim$ 1 $\mu$m) and a lens with 7.5 cm focal length (spot size of $\sim$ 200 $\mu$m). The lens results in much greater inhomogeneous broadening to the PL linewidth as described in the main text. Therefore, polarized PL from bare $MoS_2$ was measured with an objective to obtain optimal polarization. The $MoS_2$ sample was mounted horizontally in an optical cryostat capable of reaching 6 K (Advanced Research Systems). Polarization was measured by pumping with a CW dye laser (SpectraPhysics Matisse 2DR) with linewidth less than 20 MHz. The dye laser wavelength is tunable in the range of 600-645 nm, and the pump power on the monolayer was 200 $\mu$W. Circularly-polarized light for valley pumping was generated using a linear polarizer (LP) and a quarter waveplate (QWP). The polarized emission was resolved with a QWP-LP analyzer. The circular polarization of the reflected pump beam was measured to be greater than 99% using this setup.

Polarized PL from the MC with embedded monolayer $MoS_2$ was performed using the same dye laser setup. Distinct from the bare monolayer measurements, the pump laser was incident at an angle of $\theta = 38°$ focused onto the sample with a spot size of 300 $\mu$m (Fig. S1f) with a lens of 12.5 cm focal length. PL was collected along the normal direction (0°) with a lens of 7.5 cm focal length used for the bare monolayer measurement. The pump power used was 3 mW. This high power is necessary because the pump energy is in the reflective stopband of the MC. The lens is used in this configuration rather than an objective to reduce the angular spread collected from the cavity.

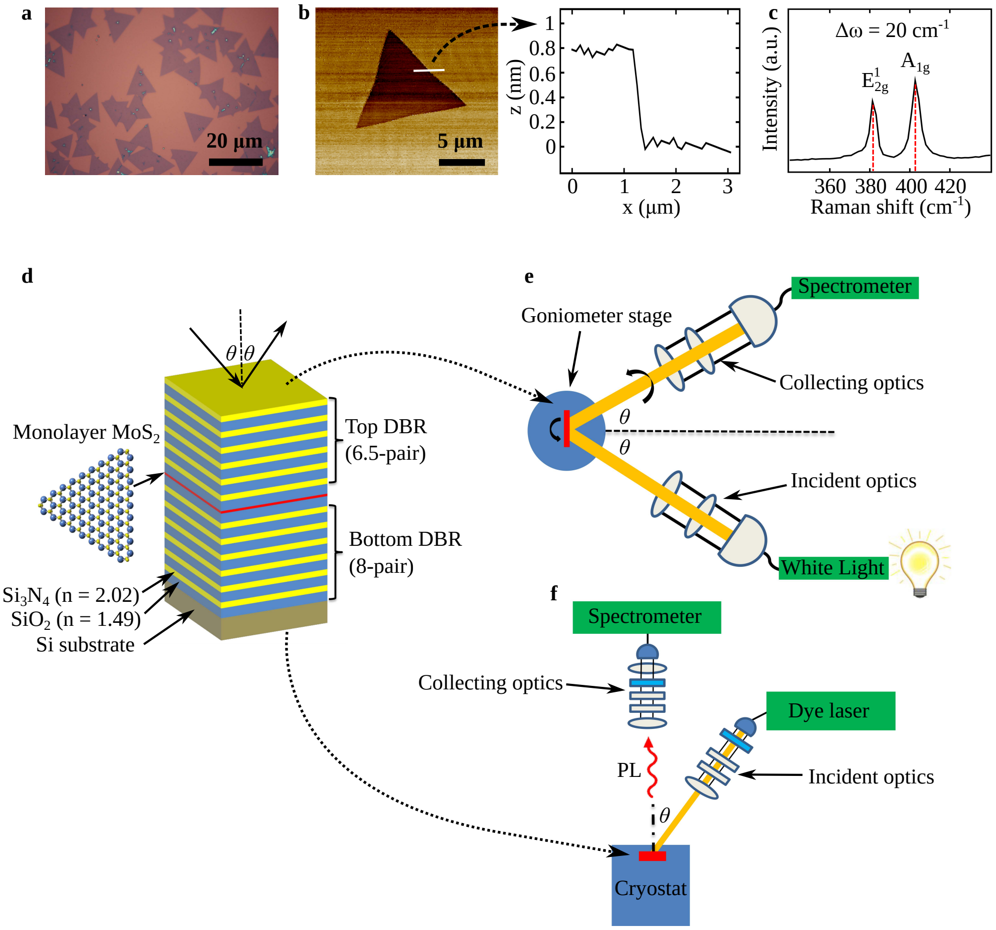


FIG. S1. **Characterization of monolayers and cavities.** **a**, Optical image of CVD-grown monolayer $MoS_2$. **b**, AFM image of CVD-grown monolayer $MoS_2$. Thickness of a monolayer is 0.8 nm (inset). **c**, Raman spectrum of CVD-grown monolayer $MoS_2$. **d**, Schematic of the MC structure. **e**, Optical setup for angle-resolved reflectivity. **f**, Optical setup for polarized PL measurement.

## III. SAMPLE PARAMETERS

The PL linewidths of the CVD grown $MoS_2$ are inhomogeneously broadened in the experimental spot size ($\Gamma_{\mathrm{ex}} \approx 90$ meV) due to the non-continuous monolayer flakes, growth seed cores, and occasional bilayer regions. The actual homogeneous exciton linewidth is narrower [5]. This is evident from the reduced linewidth $\Gamma_{\mathrm{c}} = 64$ meV when using a smaller spot size from an objective, which can be seen from Fig. 3e of the main text. The cavity linewidth $\Gamma_{\mathrm{c}}$ is also broadened by about 3-4 meV by the non-zero collection angle of the experiment since the cavity energy in angle dependent.

Estimates of the cavity QED coupling $g$ are from the standard cavity models [6, 7] using the inhomogeneous linewidths rather than the unmeasured exciton homogeneous linewidth. The coupling meets the necessary conditions for strong coupling [6] $2g > |\gamma_{\mathrm{ex}} - \gamma_{\mathrm{c}}|$, where $\gamma = \Gamma/2$. Accounting for the narrower homogeneous linewidth would change the reported coupling $g$, but move the system further into the strong coupling regime. The analysis of the manuscript, and the existence of exciton-polariton quasiparticles evidenced by the Rabi splitting, is not influenced by the ambiguity in the exicton-photon coupling constant $g$ since the results are in the high cooperativity limit. Using different TMD materials with narrower emission could result in stronger coupling.

Table I summarizes parameters for five measured MC-$MoS_2$ samples. All the linewidths for bare $MoS_2$ $A$-exciton ($\Gamma_{\mathrm{ex}}$) are the inhomogeneously broadened $\Gamma \sim 90$ meV. Sample 1, with cavity energy resonant with the $MoS_2$ exciton energy, was used for the emission polarization in the main text. Sample 2 is a similar sample confirming reproducibility, with supporting data in section IV. Sample 3 was used for the off-resonant Rabi splitting measurement in Fig. 2b,c,d in the main text. Sample 4 and 5 are additional samples demonstrating the quasi-strong coupling regime.

| Sample | DBR layers *Top* | DBR layers *Bottom* | $E_{\mathrm{ex}} - E_{\mathrm{c}}$ (meV) | $\hbar\Omega_{\mathrm{Rabi}}$ (meV) | $\hbar\Gamma_{\mathrm{c}}$ (meV) | $\hbar g$ (meV) |
|---|---|---|---|---|---|---|
| 1 | 5.5 | 7 | 0 | 20 | 8 | 23 |
| 2 | 6.5 | 8 | 0 | 24 | 7 | 24 |
| 3 | 5.5 | 6 | 21 | 39 | 10 | 28 |
| 4 | 5.5 | 6 | 20 | 33 | 10 | 26 |
| 5 | 4.5 | 5 | 15 | 23 | 20 | 21 |

TABLE I. Measured MC-$MoS_2$ samples.

## IV. SUPPORTING DATA

### A. Coupling of polarization into MC

For valley polarization measurements, an angle $\theta = 38°$ was used for all pump wavelengths ranging from 600 to 645 nm. The different reflections for linear polarization in and out of the plane result in imperfect excitation of polarization in the cavity mode, which is especially significant for light on resonance with the cavity. Figure S2 shows the intracavity polarization at $\theta = 38°$ obtained from multilayer electromagnetic simulations. For this angle, the MC resonance is at 631.8 nm. The efficiency of pumping intracavity circular polarization degrades near resonance since the external pump has different reflection coefficients for $s$ and $p$ polarizations. Off-resonance, the difference between $s$ and $p$ polarizations is minimal; across the range $600 - 645$ nm in 5 nm steps, the intracavity field is expected to maintain $p > 88\%$. For these wavelengths, the pump is never on resonance with the cavity so most pump power is reflected from the top DBR.

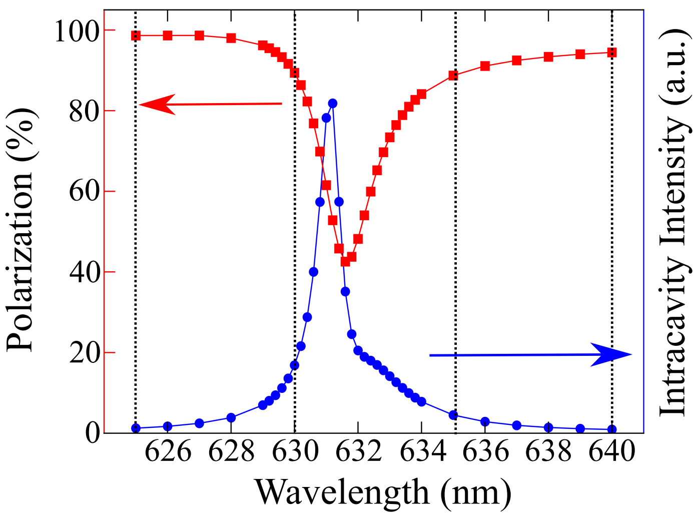


FIG. S2. **Pump polarization in the MC.** For a pump incident at $\theta = 38°$, the effective polarization of the intracavity field and its relative intensity are shown from electromagnetic simulations. The black dotted lines denote our choice of pump photon wavelengths for the experimental data plotted in the main text.

## B. Reproducibility

Figures S3, S4, and S5 show data collected from Sample 2 from Table I to confirm the effects reported in the manuscript. Dependence of the polarized emission on the pump energy $E_{\mathrm{ph}}$ measured on Sample 2 is shown in Fig. S3. UP, LP and D represent the upper polariton, the lower polariton and the emitting defect state. At 6 K, the maximum polarization is greater than that at room temperature, consistent with the trends known from bare monolayer $MoS_2$ emission [8–11]. The defect emission remains unpolarized regardless of $E_{\mathrm{ph}}$, confirming that the observed polarization arises from the dynamics of the exciton state and not from a bias in the experimental apparatus or measurement scheme.

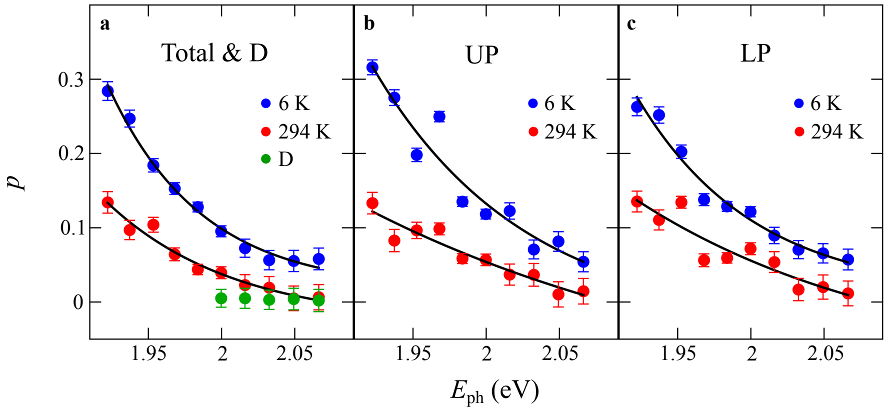


FIG. S3. **Energy-dependent emission polarization of MC-$MoS_2$.** Spectrally-integrated emission polarization $p$ of the total PL emission, the defect state, and the UP and LP modes at 6 K and 294 K. The LP and UP modes are fit to peak functions separate their relative weights. The exponential decay fit for $p$ is a guide to the eye.

## C. Representative Spectra from Second MC-$MoS_2$ Sample

Representative spectra at 6 K are shown in Fig. S4, in analogy with data shown in the manuscript.

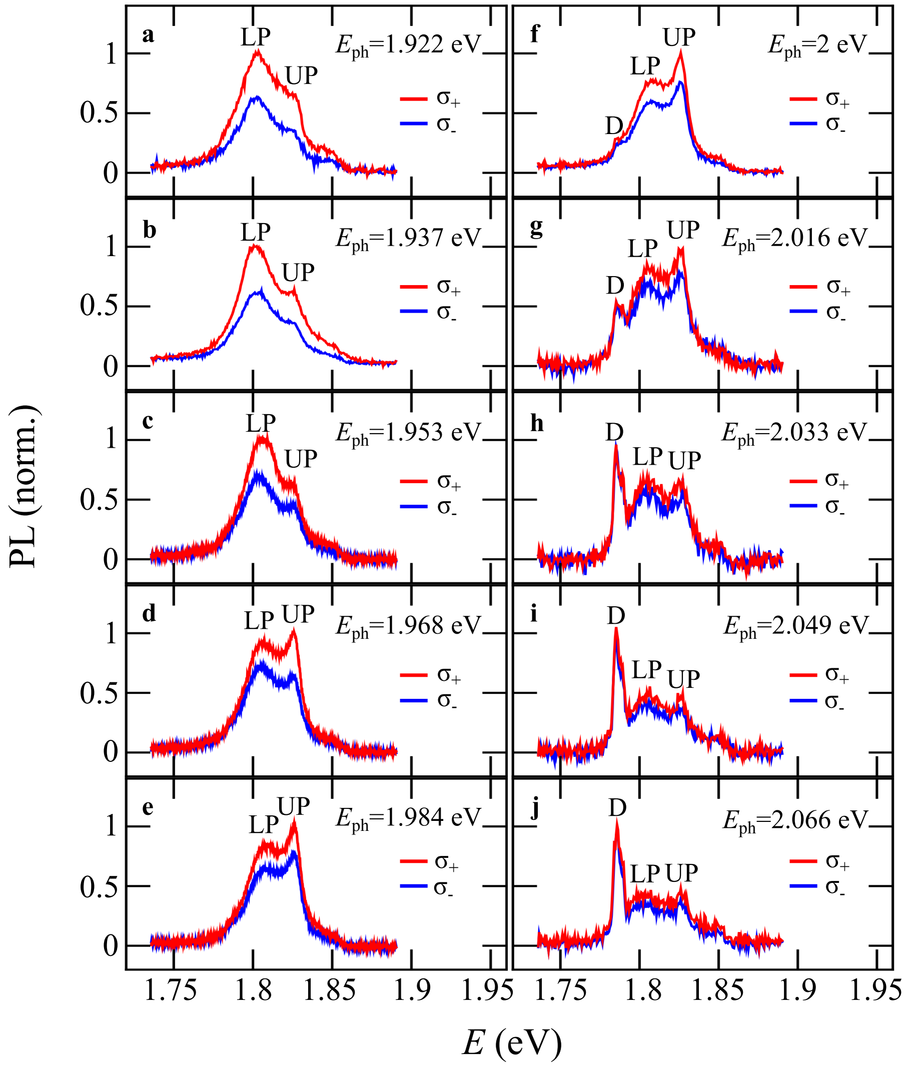


FIG. S4. **Energy-dependent emission spectra of MC-$MoS_2$.** Polarized emission spectra of MC-$MoS_2$ at 6 K with $E_{ph}$ = 1.922 to 2.066 eV. For $E_{ph}$ = 2.066 − 2 eV, low-energy defect emissions are observed.

### D. Polarization Temperature Dependence

Figure S5 shows temperature-dependent evolution of emission polarization $p$ from the on-resonant Sample 2. This is in analogy to the results reported for Sample 1 in Fig. 4 of the main text. Both near resonant ($E_{\mathrm{ph}}$ = 1.922 eV) and off-resonant ($E_{\mathrm{ph}}$ = 1.984 eV) pumping energy is shown, with a distinct increase in 6 K polarization for lower energy. As shown in Fig. S3, the UP, LP and the total emission all have very similar polarizations and here we only show the total emission polarization. The $p$ of bare $MoS_2$ for $E_{\mathrm{ph}}$ = 1.984 eV is similarly distinctly smaller than that for $E_{\mathrm{ph}}$ = 1.922 eV. Following the same procedure as with the Sample 1 data (Fig. 4 in the main text), the fits give $\Gamma_c = 4.2$ ($E_{\mathrm{ph}}$ = 1.984 eV) and 4.6 ($E_{\mathrm{ph}}$ = 1.922 eV). The fit quality and similar extracted parameters are consistent with the results from the main text. This repeatability confirms the validity of our valley-sensitive cavity measurements and modeling.

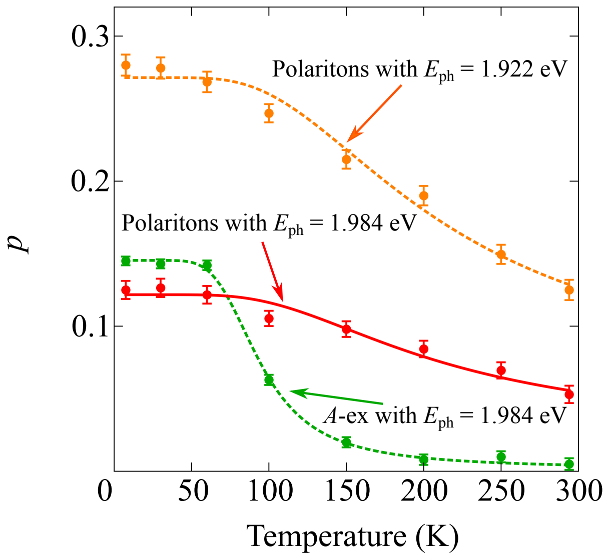


FIG. S5. **Temperature-dependent emission polarization of bare $MoS_2$ and MC-$MoS_2$ from Sample 2.** Spectrally-integrated emission polarization $p$ of the total PL emission from the MC-$MoS_2$ and the bare $MoS_2$ $A$-excitons.

## V. INTERPRETING POLARIZATION DYNAMICS

### A. Basic rate model for polarized luminescence

The valley polarization dynamics of bare monolayer $MoS_2$ is typically understood from standard rate equation models [8]. A version of this model is reproduced here for completeness. Here, $n_1$ ($n_2$) represents the exciton population of the $K$ ($K'$) valley. Simple rate equations for the exciton populations of each of the $K$ and $K'$ valleys can be written as

$$\frac{dn_{1(2)}}{dt} = P_{1(2)\mathrm{in}} - \frac{n_{1(2)}}{\tau_{\mathrm{ex}}} \pm \frac{n_2 - n_1}{\tau_{\mathrm{v}}} \tag{S1}$$

Here, $P_{1(2)\mathrm{in}}$ are the pumping rates of each valley, $\tau_{\mathrm{ex}}$ is the exciton decay rate, and $\tau_{\mathrm{v}}$ is the intervalley scattering rate. When the system is in equilibrium, $dn_{1(2)}/dt = 0$. We will assume that the $K$ valley is being pumped with rate $P_{1\mathrm{in}}$. Since valley pumping for general $E_{\mathrm{ph}}$ is not perfect, we will assume that $P_{2\mathrm{in}} = \alpha P_{1\mathrm{in}}$ with $\alpha$ a ratio describing the relative efficiency of valley pumping. Since the experimental pump has 99% circular polarization, the $\alpha \neq 0$ in the bare monolayer originates from intrinsic exciton absorption and relaxation features of the material.

The bare monolayer emission polarization is defined as $p_{\mathrm{bare}} = \frac{n_1 - n_2}{n_1 + n_2}$, and can be solved from the rate equations:

$$p_{\mathrm{bare}} = \left(\frac{1-\alpha}{1+\alpha}\right) \frac{1}{1 + 2\tau_{\mathrm{ex}}/\tau_{\mathrm{v}}} = \frac{A}{1 + 2\Gamma_{\mathrm{v}}/\Gamma_{\mathrm{ex}}} \tag{S2}$$

with $\Gamma_{\mathrm{v}} = 1/\tau_{\mathrm{v}}$, $\Gamma_{\mathrm{ex}} = 1/\tau_{\mathrm{ex}}$, and $A = (1-\alpha)/(1+\alpha)$. Equation S2 is what appears in the main text and is used for fitting.

### B. Valley-specific cavity QED model

The polarization temperature dynamics of MC-$MoS_2$ emission (such as in Fig. 4a of the main text and Fig. S5 in the supplementary) can be understood from a valley-specific cavity quantum electrodynamics (QED) model. We follow a master equation approach based on microcavity exciton-polariton emission theory [12]. Incorporating simple approximations to account for incoherent pumping, intervalley scattering, dissipation, and coherent exciton-photon coupling, we extend the single-cavity exciton-polariton model to account for the distinct exciton transitions in the two distinct valleys of monolayer TMDs (Fig. S6).

Exciton fields in two different valleys, $K$ and $K'$, are each individually and coherently coupled to their own circularly-polarized cavity mode, $a_1$ and $a_2$, with the coupling strength, $g$. The $a_1$ and $a_2$ modes represent the degenerate, linearly-independent *circularly-polarized* photon modes in the MC, and similar $b_1$ and $b_2$ modes describe the exciton fields in each valley. For cavity mirrors with similar $s$ and $p$ reflection coefficients and linewidth larger than any splitting between two modes, this is a reasonable approximation. The Hamiltonian

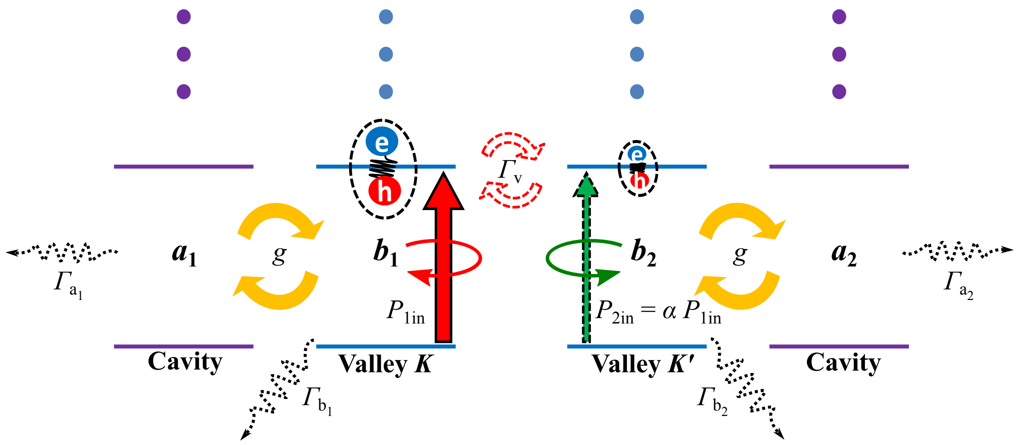


FIG. S6. **Valley-specific cavity QED.** Schematic of exciton and photon energy levels for describing light-matter interactions in MC with embedded monolayer $MoS_2$. The scheme includes incoherent pumping ($P_{1,2\text{in}}$), incoherent intervalley scattering ($\Gamma_\text{v}$), dissipation ($\Gamma_{a_1,a_2}$, $\Gamma_{b_1,b_2}$), and coherent exciton-photon coupling ($g$).

for this system can be written as

$$H/\hbar = \omega_{a_1} a_1^\dagger a_1 + \omega_{a_2} a_2^\dagger a_2 + \omega_{b_1} b_1^\dagger b_1 + \omega_{b_2} b_2^\dagger b_2 + g(a_1^\dagger b_1 + a_1 b_1^\dagger) + g(a_2^\dagger b_2 + a_2 b_2^\dagger) \tag{S3}$$

Here, $a_1(a_1^\dagger)$ and $a_2(a_2^\dagger)$ are lowering (raising) operators for the circularly-polarized cavity photon modes and $b_1(b_1^\dagger)$ and $b_2(b_2^\dagger)$ are lowering (raising) operators for excitons in the $K$ and $K'$ valleys. Since small populations of exciton-polaritons in a MC are a bosonic system (when interparticle interactions are ignored), these operators obey the harmonic oscillator commutation relation, $\left[O, O^\dagger\right] = 1$. The energies $\hbar\omega_{a_1}$, $\hbar\omega_{a_2}$, $\hbar\omega_{b_1}$, and $\hbar\omega_{b_2}$ are the transition energies for the MC photons and the valley-specific excitons. Since the cavity mode emission is collected on resonance with the $k = 0$ exciton in the experiment, we will treat the transition energies to all be equal in this analysis ($\omega_{a_1} = \omega_{a_2} = \omega_{b_1} = \omega_{b_2}$).

Whereas Eq. (S3) describes the coherent interactions, valley pumping and dissipation are incoherent processes. External pumping with circularly-polarized ($\sigma_+$) incident photons with energy higher than the excitonic bandgap and cavity resonance will create hot excitons preferentially populating the $K$ valley. These hot excitons will relax to the energy minimum near $k = 0$, which will consist of exciton-polariton modes due to the resonant coupling with the MC. Subsequent exciton recombination results in photon emission with $k_\parallel = 0$ at 0°, which is collected by the optical setup. Because of the hot exciton generation and subsequent incoherent relaxation, high-energy $\sigma_+$ pumping to a single valley (such as $K$) is not perfect. As with the bare monolayer rate equations in Sec. V A, this undesired $K'$ pumping is accounted for by the ratio $\alpha$: $P_{2\text{in}} = \alpha P_{1\text{in}}$. In addition to the external pumping, we include an incoherent intervalley scattering proportional to the instantaneous expectation values of exciton numbers, $n_{b_{1(2)}} = b_{1(2)}^\dagger b_{1(2)}$ and the intervalley scattering rate, $\Gamma_\text{v}$. Therefore, the total incoherent pumping of each valley exciton mode can be expressed as

$$P_{1(2)} = P_{1(2)\text{in}} + \Gamma_\text{v} n_{2(1)} \tag{S4}$$

For the dissipation, cavity decay rates are $\Gamma_{a_1,a_2} = \Gamma_\mathrm{c} = 2\kappa$, where $\kappa$ is the intrinsic half width at half maximum linewidth of the MC and $\Gamma_\mathrm{c}$ is the full width. The exciton decay rate in each valley is expressed as $\Gamma_{b_1,b_2} = \Gamma_\mathrm{ex} + \Gamma_\mathrm{v}$ which is the sum of the radiative relaxation rate, $\Gamma_\mathrm{ex} = 2\gamma$, and the intervalley scattering rate ($\gamma$ is the field decay rate).

The emission from this system are studied using a steady-state master equation approach with the Hamiltonian in Eq. (S3). The time-derivative of the density matrix $\rho$ is found from the master equation $\partial_t\rho = \mathcal{L}\rho$ where $\mathcal{L}\rho$ is the Liouvillian superoperator. Incoherent dissipation and pumping are included using the standard Lindblad form for each mode [12]. Assuming no external pumping of the MC $a$ and $b$ modes, the full master equation for the model outlined in Fig. S6 is then expressed as [12]

$$\begin{aligned}\partial_t\rho = \mathcal{L}\rho = &\frac{i}{\hbar}[\rho, H]\\ &+ \sum_{c=a_1,a_2} \frac{\Gamma_\mathrm{c}}{2}(2c\rho c^\dagger - c^\dagger c\rho - \rho c^\dagger c)\\ &+ \sum_{c=b_1,b_2} \frac{\Gamma_\mathrm{c}}{2}(2c\rho c^\dagger - c^\dagger c\rho - \rho c^\dagger c) + \frac{P_\mathrm{c}}{2}(2c^\dagger\rho c - cc^\dagger\rho - \rho cc^\dagger)\end{aligned} \tag{S5}$$

Here, each of the two cavity modes have decay terms and the two valley-specific excitons have both pumping and decay terms. $\Gamma_\mathrm{c}$ represents the associated decay rate and $P_\mathrm{c}$ is the associated pumping rate of the $c = a_1, a_2, b_1$, or $b_2$ modes.

The expectation value of an observable $A$ can be calculated as $\langle A\rangle = \mathrm{Tr}(A\rho)$ and its time dependence as $\partial_t\langle A\rangle = \mathrm{Tr}(A\partial_t\rho) = \mathrm{Tr}(A\mathcal{L}\rho)$. For the purely bosonic system, the two-field operator expectation values form a closed 16-vector basis for a system of rate equations:

$$\begin{aligned}\partial_t\langle A\rangle = &-\frac{i}{\hbar}\langle [A, H]\rangle\\ &+ \sum_{c=a_1,a_2} \frac{\Gamma_\mathrm{c}}{2}\left\langle 2c^\dagger Ac - Ac^\dagger c - c^\dagger cA\right\rangle\\ &+ \sum_{c=b_1,b_2} \frac{\Gamma_\mathrm{c}}{2}\left\langle 2c^\dagger Ac - Ac^\dagger c - c^\dagger cA\right\rangle + \frac{P_\mathrm{c}}{2}\left\langle 2cAc^\dagger - Acc^\dagger - cc^\dagger A\right\rangle\end{aligned} \tag{S6}$$

where $\langle A\rangle$ are $n_{a_1}$, $n_{a_2}$, $n_{b_1}$, $n_{b_2}$, $n_{a_1a_2}$, $n_{a_2a_1}$, $n_{a_1b_1}$, $n_{b_1a_1}$, $n_{a_1b_2}$, $n_{b_2a_1}$, $n_{a_2b_1}$, $n_{b_1a_2}$, $n_{a_2b_2}$, $n_{b_2a_2}$, $n_{b_1b_2}$, and $n_{b_2b_1}$,. Note that $n_{a_1} = \left\langle a_1^\dagger a_1\right\rangle$, $n_{a_1a_2} = \left\langle a_1^\dagger a_2\right\rangle$, and so on. The observables from the MC-$MoS_2$ system can be calculated from the steady-state solutions of this system of 16 first-order differential equations. The inclusion of incoherent scattering as a new term in Eq. S4 propagates to a nonlinear coupling in the time evolution expectation values in Eq. (S6). This procedure is an approximation to obtain rate equations with incoherent scattering from the master equation in the limit of small populations. We do not argue for general validity of this approach to the master equation formalism, and this approach neglects the phonon bath that would mediate this incoherent scattering. A full master equation theory would treat the incoherent scattering as a coupling mechanism. Here, we proceed assuming the rate equations of Eq. (S6) with the nonlinear incoherent coupling term are sufficiently accurate for weak fields to describe the coupled light-matter dynamics.

Eq. (S2) for the polarization $p_{\text{bare}}$ of PL emission from bare $MoS_2$ can be recovered from this model for $g = 0$. For the MC embedded with $MoS_2$ explored in the main text, the $k_{\parallel} = 0$ emission does not directly come from omnidirectional incoherent exciton decay but rather through directional emission from the cavity-coupled exciton-polaritons. Emitted resonant photons must exit the MC system to the collection optics through the two circularly-polarized cavity modes $a_1$ and $a_2$, and thus the emission is proportional to cavity populations $n_{a_1}$ and $n_{a_2}$ rather than $n_{b_1}$ and $n_{b_2}$ (in strong coupling this distinction is irrelevant since the $a_i$ and $b_i$ populations are identical). The polarization of light collected from the MC experiment differs from $p_{\text{bare}}$ and is not directly calculated from the valley populations:

$$p_{\text{MC}} = \frac{n_{a_1} - n_{a_2}}{n_{a_1} + n_{a_2}} \tag{S7}$$

Using steady-state solutions for $n_{a_1}$ and $n_{a_2}$ in the low pump power limit ($P_{1\text{in}}$, $P_{2\text{in}} \to 0$),

$$p_{\text{MC}} = \left(\frac{1-\alpha}{1+\alpha}\right)\left(\frac{2C(1+\frac{\Gamma_c}{\Gamma_{ex}}) + (1+\frac{\Gamma_v}{\Gamma_{ex}}+\frac{\Gamma_c}{\Gamma_{ex}})}{2C(1+\frac{\Gamma_c}{\Gamma_{ex}}+\frac{2\Gamma_v}{\Gamma_{ex}}) + (1+\frac{2\Gamma_v}{\Gamma_{ex}})(1+\frac{\Gamma_v}{\Gamma_{ex}}+\frac{\Gamma_c}{\Gamma_{ex}})}\right) \tag{S8}$$

where $C = 2g^2/\Gamma_{ex}\Gamma_c$ is the equivalent of the single-atom cooperativity from cavity QED. We can simplify Eq. (S8) to Eq. (3) in the main text,

$$p_{\text{MC}} = \left(\frac{1-\alpha}{1+\alpha}\right)\frac{1}{1+\frac{2\Gamma_v}{\Gamma_{ex}+\Gamma_c}} = \frac{A}{1+\frac{2\Gamma_v}{\Gamma_{ex}+\Gamma_c}} \tag{S9}$$

since the second term of Eq. (S8), $2C$ is much greater than 1, $\Gamma_c/\Gamma_{ex}$, and $\Gamma_v/\Gamma_{ex}$. Here, $A$ is a proportionality fit constant as introduced in Eq. S2.

The cooperativity condition is met across the temperature range of our experiments. For our analysis, $\hbar g \sim 20$ meV is taken from our measured coupling constant of monolayer $MoS_2$ (Fig. 2b in the main text). $\hbar\Gamma_c \sim 4$ meV is the intrinsic full width at half maximum linewidth of the MC which is derived from the measured linewidth (7 meV) by accounting for the Gaussian spread of incident angle of light rays in the Gaussian beam. $\hbar\Gamma_{ex} = 0.16$ meV is calculated from the total exciton decay time $\tau_{ex} = 4$ ps from time-resolved PL measurements [13], which is different from the broad $MoS_2$ PL linewidth of 90 meV which is mostly dominated by the inhomogeneity of the materials and the homogeneous exciton-phonon broadening [5, 14, 15]. $g$, $\Gamma_c$, and $\Gamma_{ex}$ are assumed to be independent of temperature. The intervalley scattering $\Gamma_v = 1/\tau_v$ is assumed to follow a thermal activation profile fit to the bare monolayer polarization as described in the main text. The high cooperativity and the low pumping power lead to a symmetry of the cavity and exciton operators such that $p_{\text{MC}}$ is equivalent to $p_{\text{bare}}$ in this regime.

### C. Fit procedure for temperature dynamics

The temperature-dependent $p_{\text{MC}}$ is fit with Eq. (S9) (in Fig. 4a in the main text as well as Fig. S5 for Samples 1 and 2, respectively). Only $\alpha$ (or $A$) and $\Gamma_c$ are free, temperature independent parameters. The bare $MoS_2$ curve is fit with Eq. (S2) to find the energy $E$

that parameterizes the phenomenological thermal activation energy for exciton recombination. This is then used to fit the MC-$MoS_2$ temperature dependence data. The only free parameters for the MC-$MoS_2$ are fits $\Gamma_c$ and the zero-$T$ polarization $A$. For Sample 1, we find $A_{UP} = 0.185 \pm 0.004$ and $\hbar\Gamma_{c,UP} = 4.2 \pm 0.6$ meV and $A_{LP} = 0.286 \pm 0.005$ and $\hbar\Gamma_{c,LP} = 5.2 \pm 0.5$ meV. These cavity linewidth results $\hbar\Gamma_c = 4.2$ and 5.2 meV from the fits are consistent with the cavity linewidth of 4 meV extracted from independent measurement of the cavity reflectivity reflectance spectrum, corrected for the finite angular distribution of the Gaussian beam. This suggests that the simple Eq. (S9) is capturing the essence of the temperature dynamics of the valley-polarized exciton-polaritons in the MC-$MoS_2$ system.

## REFERENCES


[1] Lee, Y.-H. *et al.* Synthesis of large-area $MoS_2$ atomic layers with chemical vapor deposition. *Adv. Mater.* **24**, 2320–2325 (2012).

[2] Lin, Y.-C., Jin, C., Lee, J.-C., Jen, S.-F., Suenaga, K. & Chiu, P.-W. Clean transfer of graphene for isolation and suspension. *ACS Nano* **5**, 2362–2368 (2011).

[3] Park, H. J., Meyer, J., Roth, S. & Skákalová, V. Growth and properties of few-layer graphene prepared by chemical vapor deposition. *Carbon* **48**, 1088–1094 (2010).

[4] Wood, J. D. *et al.* Annealing free, clean graphene transfer using alternative polymer scaffolds. *Nanotechnology* **26**, 055302 (2015).

[5] Moody, G. *et al.* Intrinsic homogeneous linewidth and broadening mechanisms of excitons in monolayer transition metal dichalcogenides. *Nature Commun.* **6**, 8315 (2015).

[6] Savona, V., Andreani, L., Schwendimann, P. & Quattropani, A. Quantum well excitons in semiconductor microcavities: unified treatment of weak and strong coupling regimes. *Sol. St. Commun.* **93**, 733–739 (1995).

[7] Deveaud, B. *The physics of semiconductor microcavities* (John Wiley & Sons, 2007).

[8] Mak, K. F., He, K., Shan, J. & Heinz, T. F. Control of valley polarization in monolayer $MoS_2$ by optical helicity. *Nature Nanotech.* **7**, 494–498 (2012).

[9] Zeng, H., Dai, J., Yao, W., Xiao, D. & Cui, X. Valley polarization in $MoS_2$ monolayers by optical pumping. *Nature Nanotech.* **7**, 490–493 (2012).

[10] Sallen, G. *et al.* Robust optical emission polarization in $MoS_2$ monolayers through selective valley excitation. *Phys. Rev. B* **86**, 081301 (2012).

[11] Wu, S., Huang, C., Aivazian, G., Ross, J. S., Cobden, D. H. & Xu, X. Vapor-solid growth of high optical quality $MoS_2$ monolayers with near-unity valley polarization. *ACS Nano* **7**, 2768–2772 (2013).

[12] Laussy, F. P., Del Valle, E. & Tejedor, C. Luminescence spectra of quantum dots in microcavities. I. Bosons. *Phys. Rev. B* **79**, 235325 (2009).

[13] Lagarde, D., Bouet, L., Marie, X., Zhu, C., Liu, B., Amand, T., Tan, P. & Urbaszek, B. Carrier and polarization dynamics in monolayer $MoS_2$. *Phys. Rev. Lett.* **112**, 047401 (2014).

[14] Rudin, S., Reinecke, T. & Segall, B. Temperature-dependent exciton linewidths in semiconductors. *Phys. Rev. B* **42**, 11218 (1990).

[15] Wei, G., Czaplewski, D. A., Lenferink, E. J., Stanev, T. K., Jung, I. W. & Stern, N. P. Size-tunable monolayer semiconductor quantum dots (2015). arXiv:1510.09135.
